# Supplementary material for: Learning Payment-Free Resource Allocation Mechanisms
Source: arXiv:2311.10927 source file (2024-08-14)
Supplement: Supplementary file 1 [file Appendix_DistributionMismatch.tex]

\section{Proof of Theorem~\ref{lem:dist_mismatch}}\label{sec:dist_mismatch}

It is obvious that the exploitability of any mechanism at agent $i$ cannot exceed the utility of agent $i$ when its demands are fully satisfied. This means for any mechanism $f$ and $v\in\Vcal,x\in\Dcal,b\in\Bcal$, we have
\begin{align}
    \exploitability_i(f,v,x,b)\leq \sum_{m=1}^{M}v_{i,m}x_{i,m} \leq M\,\overline{v}\,\overline{x},\label{lem:dist_mismatch:proof_eq1}
\end{align}
where the second inequality is due to the boundedness of values and demands.

Let $p_F$ and $p_{F'}$ denote the probability density function associated with $F$ and $F'$. We have for any $i$
\begin{align*}
    &E_{(v,x,b)\sim F}[\exploitability_i(f,v,x,b)]\notag\\
    &=E_{(v,x,b)\sim F'}[\exploitability_i(f,v,x,b)] \notag\\ &\hspace{20pt}+\Big(E_{(v,x,b)\sim F}[\exploitability_i(f,v,x,b)]\notag\\ 
    &\hspace{40pt}-E_{(v,x,b)\sim F'}[\exploitability_i(f,v,x,b)]\Big) \notag\\
    &\leq\epsilon \hspace{-2pt}+\hspace{-2pt} \int \hspace{-2pt} \exploitability_i(f,v,x,b)\left(p_{F'}(v,x,b)\hspace{-2pt}-\hspace{-2pt}p_{F}(v,x,b)\right) dv\,dx\,db\notag\\
    &\leq\epsilon \hspace{-2pt}+\hspace{-2pt} \int \hspace{-3pt}|\exploitability_i(f,v,x,b)|\hspace{-1pt}\left|p_F(v,x,b)\hspace{-2pt}-\hspace{-2pt}p_{F'}(v,x,b)\right| dv\,dx\,db\notag\\
    &\leq \epsilon + M\,\overline{v}\,\overline{x}\int \left|p_F(v,x,b)-p_{F'}(v,x,b)\right| dv\,dx\,db\notag\\
    &=\epsilon + 2M\,\overline{v}\,\overline{x}d_{TV}(F,F'),
\end{align*}
where the third inequality applies \eqref{lem:dist_mismatch:proof_eq1} and the final equation comes from the definition of TV distance, i.e. for any distribution $F_1, F_2$ over $\Xcal$
\[d_{TV}(F_1,F_2)=\frac{1}{2}\int_{\Xcal} \left|p_F(x)-p_{F'}(x)\right| dx.\]

\qed
