# Supplementary material for: Learning Payment-Free Resource Allocation Mechanisms
Source: arXiv:2311.10927 source file (2024-08-14)
Supplement: Supplementary file 2 [file Appendix_RelatedWork.tex]

\section{Related Works}
\noindent\textbf{One-shot allocation without payment:} 
\cite{GuoContizer} consider the problem of dividing multiple divisible goods between $2$ agents and show that any IC mechanism achieves at most $0.841$ of the optimal social welfare in the worst case (defined as an overall utility of all agents). \cite{10.1007/978-3-642-25510-6_16} obtain analogous result for a more general case of $n$ agents. \cite{cole2013mechanism} prove that no IC mechanism can guarantee to every agent a fraction of their proportionally fair allocation greater than $\frac{n+1}{2n}$, and provide a partial allocation (PA) mechanism that allocates to each agent a fraction of the corresponding PF allocation. \\ %We consider a slightly more general setup than~\cite{cole2013mechanism}, and learn mechanisms that fall between the extremes of PF and PA allocations.\\
\noindent\textbf{Auction design/resource allocation with payment:}
% When monetary transfers from the agents to the supplier are allowed as a way to ensure truthful reporting, \cite{dütting2022optimal, ivanov2022optimal} adopt a learning-based framework similar to the one in our paper. 
When payments from the agents to the supplier are allowed, \cite{SL08,Rou10,BGM22} design sophisticated monetary transfer schemes that ensure truthful reporting. More recently, \cite{dütting2022optimal,ivanov2022optimal} adopt a learning-based framework similar to the one in our paper.
% The authors in \cite{dütting2022optimal} introduce a neural-network-parameterized mechanism, \texttt{RegretNet}, that explores a regret-based approach in order to relax the requirement on truthfulness and thus approximate optimal auctions.
A neural-network-parameterized mechanism, \texttt{RegretNet}, is proposed in \cite{dütting2022optimal}, which determines the price of a resource with the aim of increasing supplier's revenue while guaranteeing the approximate truthfulness of the agents.
Our work is partially inspired by this approach.\\
% , in that, we relax truthfulness requirement while learning fractional fair allocations without money. 
{\noindent\textbf{Approximate incentive compatibility in ML:} \cite{DFP10} consider regression learning where the  global goal is to minimize average loss in the setting of strategic agents that might misreport their values over the input space. When payments are disallowed, they present a mechanism which is approximately IC and optimal for the special case of the buyer's utilities being defined by the absolute loss.
More recently, \cite{NEURIPS2020_ae87a54e} focus on learning linear classifiers, when the training data comes in online manner from the strategic agents who can misreport the feature vectors, and propose an algorithm that exploits the geometry of the learner's action space. 
% in order to guide learning towards their preferred function
