# Supplementary material for: Learning Payment-Free Resource Allocation Mechanisms
Source: arXiv:2311.10927 source file (2024-08-14)
Supplement: Supplementary file 3 [file Appendix_TruthfulMecNotPF.tex]

\clearpage
\section{Proportional Fairness $\&$ Truthfulness}

\begin{definition}
An allocation~$s^* \in \mathcal{S}$ is proportionally fair if, for any other allocation~$s' \in \mathcal{S}$, the aggregate proportional change to the valuations after replacing~$s^*$ with~$s'$ is not positive, i.e, for any valuation~$v$
\[
\sum_{i} \frac{[u_i(s',v) - u_i(s^*,v)]}{u_i(s^*,v)} \leq 0.
\]
\end{definition}

Consider a simple case of unit budget and infinite demand with~$M$ divisible resources and~$N$ agents.  Let~$\mathcal{S}$ denote the set of all allocations, i.e, $\mathcal{S} = \{s | s_{ij} \geq 0,~\text{and}~\sum_{i}s_{ij} \leq 1 \}$. 

\begin{lemma}
   Let~$M=2$, $N=2$ and $w = \boldsymbol{1}$. No truthful mechanism can obtain a PF solution.
\end{lemma}

\begin{proof}
We will show the proof by contradiction. Suppose there exists a truthful mechanism,~$T^*$, that is proportionally fair. 

Let~$v_1$ and $v_2$ denote the (non-negative) valuations of the two agents such that $\sum_j v_{ij} =1$. The utility functions are denoted as~$u_1(T,v_1)$ and $u_2(T,v_2)$ for any mechanism~$T(v_1,v_2) \in \mathcal{S}$. Clearly, the utility derived by both agents is non-negative, i.e, 
\[u_1(T,v_1) \geq 0,~\text{and}~ u_2(T,v_2) \geq 0. \]
Since~$T^*$ is proportionally fair, by definition, $\forall~s' \in \mathcal{S}$, 
\[
\sum_{i} \frac{[u_i(s',v_1) - u_i(T^*,v_i)]}{u_i(T^*,v_i)} \leq 0.
\]
This implies that
\[
\frac{[u_1(s',v_1) - u_1(T^*,v_1)]}{u_1(T^*,v_1)} + \frac{[u_2(s',v_2) - u_2(T^*,v_2)]}{u_2(T^*,v_2)} \leq 0.
\]
Rearranging, we have
\[
\frac{u_2(T^*,v_2)}{u_1(T^*,v_1)} \leq \frac{[u_2(T^*,v_2) - u_2(s',v_2)]}{[u_1(s',v_1) - u_1(T^*,v_1)]}.
\]
Suppose \textit{both} agents misreport. Since the mechanism~$T^*$ is truthful, misreporting leads to allocation such that, for some~$\epsilon_1,\epsilon_2,\epsilon_3, \epsilon_4 \geq 0$,
\[
q' = 
\begin{bmatrix}
T_{11}^* - \epsilon_1 & T_{12}^* -\epsilon_2 \\
T_{21}^* - \epsilon_3 & T_{22}^* - \epsilon_4
\end{bmatrix}.
\]
Note that $\sum_j q'_{ij} \leq 1$, so it is a valid allocation, i.e, $q' \in \mathcal{S}$. We have by rearranging, 
\[
    \frac{u_2(T^*,v_2)}{u_1(T^*,v_1)} \leq -\Bigg\{\frac{\epsilon_3 v_{21}+ \epsilon_4 v_{22}}{\epsilon_1 v_{11} + \epsilon_2 v_{12}}  \Bigg\} < 0.
\]
But this is a contradiction as the the utilities are non-negative. 
\end{proof}

\[u_1(\bar{v}_1,\bar{v}_2)\leq u_1(v_1,\bar{v}_2)\]

\[u_2(\bar{v}_1,\bar{v}_2)\leq u_2(\bar{v}_1,v_2)\]

\[u_1(\bar{v}_1,\bar{v}_2)\leq u_1(v_1,v_2)\]

\[v_1^{\top} a(\bar{v}_1,\bar{v}_2)\leq v_1^{\top} a(v_1,\bar{v}_2)\]

\[v_2^{\top} a(v_1,\bar{v}_2)\leq v_2^{\top} a(v_1,v_2)\]

\[v_1^{\top} a(\bar{v}_1,\bar{v}_2)\leq v_1^{\top} a(v_1,v_2)\]
