# Supplementary material for: Learning Payment-Free Resource Allocation Mechanisms
Source: arXiv:2311.10927 source file (2024-08-14)
Supplement: Supplementary file 5 [file Appendix_PAMechanism.tex]

\section{Partial Allocation Mechanism}\label{sec:PA}

The partial allocation mechanism, proposed in \shortciteN{cole2013mechanism}, is built upon the PF mechanism and withholds resources according to an externality ratio. Specifically, given reported valuations $v\in\mathbb{R}^{N\times M}$ and demands $d\in\mathbb{R}^{N\times M}$ across all agents and resources and budgets $b\in\mathbb{R}^M$, let $a^\star\triangleq f^{PF}(v,x,b)$ denote the allocation made by the PF mechanism.

Let $x^{-i}\in\mathbb{R}^{N\times M}$ denote a modified demand matrix where
\begin{align*}
x^{-i}_{j}=
\begin{cases}
    x_j\in\mathbb{R}^M, & i\neq j\\
    0 \in\mathbb{R}^M, & i= j
\end{cases}
\end{align*}

For each agent $i$, we calculate
\[a^{-i,\star}\triangleq f^{PF}(v,x^{-i},b),\]
which is the PF allocation outcome that would arise in the absence of agent $i$. We further compute the externality ratio $r_i\in\mathbb{R}_+$ for agent $i$ as
\[r_i=\left(\frac{\prod_{j\neq i}u_j(a^{\star},v,x)^{w_j}}{\prod_{j\neq i}u_j(a^{-i,\star},v,x)^{w_j}}\right)^{1/w_i},\]
where $u_i$ is the utility function defined in \eqref{def:utility}.

The PA mechanism allocates to agent $i$ according to the following rule
\[f_i^{PA}(v,x,b)=r_i a_i^{\star}.\]

It is easy to verify that $r_i\in[0,1]$. Therefore, the PA mechanism is always feasible. \shortciteN{cole2013mechanism}[Theorem 3.2] proves that it is also perfectly incentive compatible for any $v,x,b$.
